# Supplementary material for: The Wisdom of Partisan Crowds: Comparing Collective Intelligence in Humans and LLM-based Agents
Source: arXiv:2311.09665 source file (2024-02-16)
Supplement: Supplementary file 1 [file aggregated_analysis.tex]

\section{Aggregated Analysis Plots}\label{app:aggregated_analysis}

\begin{figure*}[htbp] % The * spans the figure across both columns
  \centering
  \includegraphics[width=0.95\linewidth]{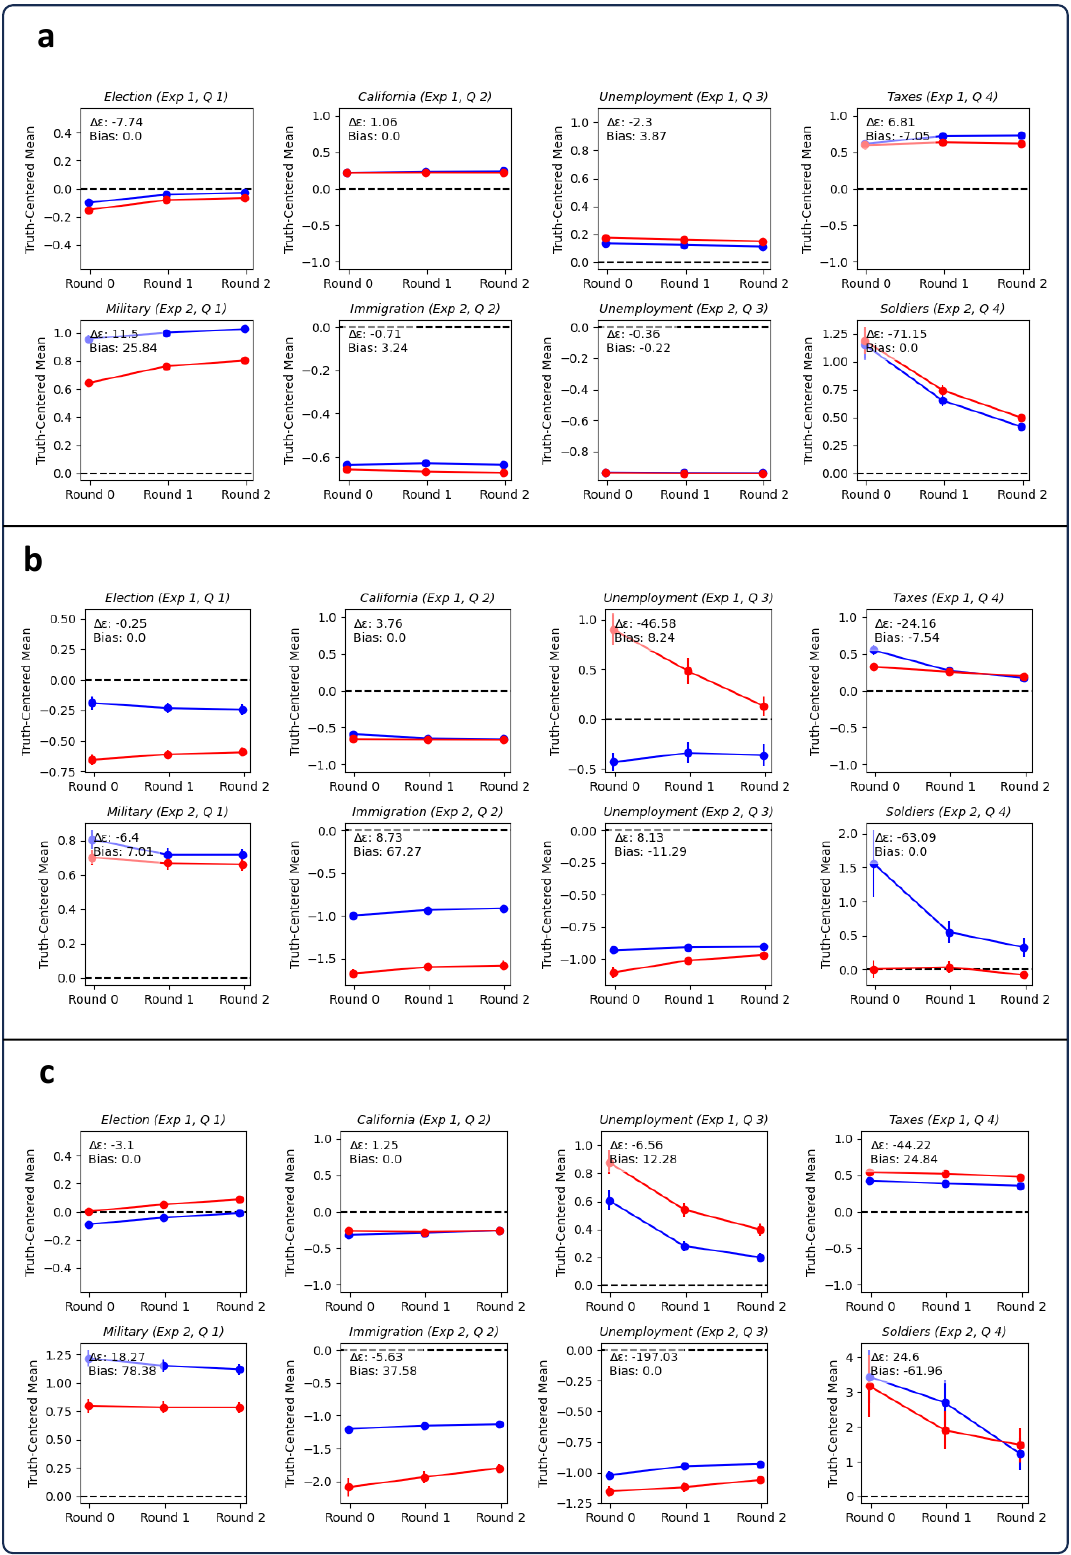}
  \caption{The normalized group mean $\eta_{p,r,q}^t$ for each question for \textbf{(a)} The detailed result for each question for Role-Playing with detailed agent personas and without Chain-of-Thought reasoning. \textbf{(b)} The detailed result for each question for Fine-tuned Role-Playing with simple agent personas and without Chain-of-Thought reasoning. \textbf{(c)} The detailed results for each question for the human data. \sn{Should reshape it to 8 rows x 3 columns matrix.}}
  \label{fig:becker_human_vs_llm_plot}
\end{figure*}

Figure~\ref{fig:becker_human_vs_llm_plot} shows the result for each question for (a) the version with the highest human alignment (role-playing without CoT reasoning), (b) fine-tuned LLM, and (c) human data from \citet{becker2019wisdom}.
